# Supplementary material for: Fast multiplexed superconducting qubit readout with intrinsic Purcell filtering
Source: arXiv:2409.04967 source file (2024-09-11)
Supplement: Supplementary file 1 [file Supplementary_H.tex]

\section{Quantum efficiency measurement}
\label{appendix:Quantum efficiency measurement}

%Removed this appendix as it is a standard measurement
